# Supplementary material for: Multilingual Reasoning Cascades Need More Context
Source: arXiv:2606.27306 source file (2026-10-19)
Supplement: Supplementary file 1 [file ablation.tex]

% \section{Ablation study}
% \label{app:ablation}
% In this section, we evaluate the individual performance effects of each component of the upstream context (original question $q_t$, English question $q_e$, and English reasoning $r_e$). \autoref{fig:llama-mistral-ablations} indicates that providing only the original question $q_t$ and English answer $a_e$ is competitive on open-ended tasks: it outperforms \cctx on three of four open-ended datasets with Mistral-7B-Instruct-v0.3 and two of four with Llama-3.1-8B-Instruct. Providing the reasoning trace \(r_e\) alongside the English
% answer \(a_e\), on the other hand, yields little improvement
% and can even degrade performance. Detailed per-dataset ablation results are provided in \autoref{app:ablation-tables}.
