# Supplementary material for: Multilingual Reasoning Cascades Need More Context
Source: arXiv:2606.27306 source file (2026-10-19)
Supplement: Supplementary file 2 [file gains_by_language_resourcedness.tex]

% \section{Gains by language resourcedness}
% \label{app:lang_resourcedness}
% We compare gains made by \cctx over \cstd on language groups of different resourcedness on datasets with a large number of languages. 
% See \autoref{fig:resourcedness} for gains on \texttt{Global-MMLU} and \texttt{Belebele}. Similar to as in \autoref{fig:ctxstd-resource}, we find that all resource regimes gain from \cctx.
% \NB{Why is this diff from the prev para? Why not combine the discussion?}

% \begin{figure}[t]
% \centering
% \includegraphics[width=\columnwidth]{latex/plots/llama_mistral_mmlu_belebele_context_minus_standard_by_resource_violin.pdf}
% \caption{Gains of the context-aware cascade (\cctx) over the standard cascade (\cstd) across resource levels on \texttt{Global-MMLU} and \texttt{Belebele} for Llama-3.1-8B-Instruct and Mistral-7B-Instruct-v0.3.}
% \label{fig:resourcedness}
% \end{figure}



% \autoref{tab:gap_closing} breaks down the share of the gap to GPT-4o-mini recovered by \cctx for each open-ended benchmark and open model. The gains are largest on Aya and smallest on BLEnD and MKQA, consistent with the pattern discussed in \autoref{sec:results}.

% \input{latex/tables/gap_closing}
