# Supplementary material for: Multilingual Reasoning Cascades Need More Context
Source: arXiv:2606.27306 source file (2026-10-19)
Supplement: Supplementary file 3 [file 8-appendix.tex]

\subsection{Results}
\input{latex/main_text/81-results}
